# Supplementary material for: Encoding word order in complex embeddings
Source: arXiv:1912.12333 source file (2020-06-28)
Supplement: Supplementary file 2 [file appendix-affine-map.tex]

\section{Proof of Claim 1 in Section 2}

Here we discuss  Claim 1 in Sec. 2. The objective is to find a linear $n$-offset transformation such that $g(\cdot)$ is bounded. Noting that all the notations in this appendix depend on the word index $j$ and arbitrary dimension $d$ which are omitted for simplifications, for example, $g_{j,d}(\cdot) \rightarrow g(\cdot)$ .



\begin{proof}
We rewrite the $n$-offset transformation as a linear format like $ g(pos+n) = w(n)g(pos) + b(n)$, in which $w$ and $b$ are two continuous functions parameterized by the offset distance $n$, $w$ is  the coefficient related to $g(pos)$ and $b$ is the constant term for $g(\cdot)$. Since $ g(pos+n) = w(n)g(pos) + b(n)$ for $\forall~n,pos \in \mathbb{R}$, it alos holds if we let $n=n_1 + n_2$:
\begin{equation}
\label{eq:n1_n2}
\begin{aligned}
    g(pos+n_1+n_2) &= w(n_1)g(pos+n_2) + b(n_1) \\
     &= w(n_1)[w(n_2)g(pos)+b(n_2)] + b(n_1) \\
     &= w(n_1)w(n_2)g(pos)+ w(n_1) b(n_2) + b(n_1) \\
\end{aligned}
\end{equation}

And by definition itself, we also have
\begin{equation}
\label{eq:n1_n2_definition}
    g(pos+n_1+n_2) = w(n_1+n_2)g(pos) + b(n_1+n_2) \\
\end{equation}

By comparing Eq.~\ref{eq:n1_n2} and Eq.~\ref{eq:n1_n2_definition}, the coefficient and the constant terms should be consistent, namely,
\begin{equation}
\label{eq:consistent}
\begin{aligned}
   w(n_1+n_2) &= w(n_1)w(n_2)   \\
   b(n_1+n_2)   &= w(n_1) b(n_2) + b(n_1) \\
     &= w(n_1)w(n_2)g(pos)+ w(n_1) b(n_2) + b(n_1) \\
\end{aligned}
\end{equation}

To first solve $ w(n_1+n_2) = w(n_1)w(n_2),~ \forall ~ n_1,n_2 \in \mathbb{R}$, we first discuss the case for $n_1,n_2 \in \mathbb{Z}^+$ as below, 
\begin{equation}
\label{eq:wn}
w(n)=  \underbrace{w(1) \times w(1) \cdots w(1)}_\text{$n$ times}  = w(1)^n.
\end{equation}
It is trivial to prove that the this valid for negative integers, i.e., $n_1,n_2 \in \mathbb{Z}^+$ by making a subtraction between $n_1$ and $n_2$ when $n_1<n_2$. 

Since the variable domain of $g(\cdot)$ was analytically extended to real-valued domain, it is necessary to discuss whether Eq.~\ref{eq:wn} still holds in the case when the position $pos$  is not a integer but a real-value number in $\mathbb{R}$, as well as $n$.  
For a $q \in \mathbb{Z}$, 
\begin{equation}
\label{eq:wn_real}
w(n)=w( \underbrace{\frac{1}{q} + \frac{1}{q} \cdots \frac{1}{q}}_\text{$q\times n$ times}) = w(\frac{1}{q})^{nq} 
\end{equation}

By considering Eq.~\ref{eq:wn} and the last term of  Eq.~\ref{eq:wn_real}, we have $w( \frac{1}{q} ) = w(1)^{\frac{1}{q}} $. To check it for any rational numbers $\frac{p}{q},\forall p,q \in \mathbb{Z}$, 
\begin{equation}
\label{eq:wn_real2}
\begin{aligned}
w(\frac{p}{q})&=w( \underbrace{\frac{1}{q} + \frac{1}{q} \cdots \frac{1}{q}}_\text{$p$ times}) = w(\frac{1}{q})^{p}  \\
&=[w(1)^{\frac{1}{q}}]^p =w(1)^{\frac{p}{q}}\\
\end{aligned}
\end{equation}
There,   Eq.~\ref{eq:wn} still holds for any rational number. Since the rationals are dense in the reals and $w$ is continuous, for any real number $r$ we can find a sequence $[r_i]$ that will converge to $r$ with $w(r_i)=f(1)^{r_i}$, so that $w(n)=w(1)^n$ for all real numbers as well.


For any given $w(\cdot)$, w(1) becomes a constant value. In order to be more general, we denote  $w(1)$ as a complex number $z_1=\alpha_1 + i \beta_1$ instead of a real number.
% \benyou{For bounded reason, discussing the domain of $\alpha$ and $\beta$}.  
The final solution for $w$ is 
\begin{equation}
\label{eq:w_solution}
w^*(n)=z_1^n
\end{equation}


Secondly, we have to solve $b(\cdot)$ by using $w^*(n)$ and $b(n_2+n_1) = w(n_1) b(n_2) + b(n_1)$. By using the similar method for solving $w(\cdot)$, 
\begin{equation}
\label{eq:w_solution}
\begin{aligned}
b(n) &= b( \underbrace{1+1 \cdots +1}_\text{n times}) \\
    &=   \underbrace{w(1)(\ldots w(1)}_\text{n-1 times} \underbrace{b(1) + b(1))+b(1)}_\text{n times} \\
    &=b(1)(1+w(1)+w(1)^2+\cdots+w(1)^{n-1}) \\
    &=b(1)(\frac{1-w(1)^n}{1-w(1)})
\end{aligned}
\end{equation}

Since $w^*(n)=z_1^n$, $w(1)=z_1$. After denoting the constant complex number $b(1)$ as $z_2=\alpha_2 + i \beta_2$.
\begin{equation}
\label{eq:b_solution}
b^*(n)= \frac{1-z_1^n}{1-z_1} z_2
\end{equation}
It is trivial to check Eq.~\ref{eq:b_solution} still holds for the case $n\in \mathbb{R}$.

By inserting the solutions for $w(\cdot)$ and $b(\cdot)$ in  $ g(pos+n) = w(n)g(pos) + b(n)$, yields
\begin{equation}
\label{eq:b_pos}
g(pos+n) =  g(pos) z_1^n + \frac{1-z_1^n}{1-z_1} z_2
\end{equation}
for $\forall pos, n \in \mathbb{R}$. Let $pos=0$ and denotes $g(0)$ as a arbitrary constant complex number $z_3=\alpha_3 + i \beta_3$, we have 

\begin{equation}
\label{eq:b_pos1}
\begin{aligned}
g(n) &=  z_3 z_1^n + \frac{1-z_1^n}{1-z_1} z_2 \\
 &=  (z_3 - \frac{z_2}{1-z_1} )  z_1^n + \frac{z_2}{1-z_1} 
\end{aligned}
\end{equation}

We can get the general solution by replacing the variable $n$ with $pos$ as below:
\begin{equation}
\label{eq:final}
g(pos) = (z_3 - \frac{z_2}{1-z_1} )  z_1^{pos} + \frac{z_2}{1-z_1} .
\end{equation}

For a specific case when $z_2=0$, i.e., $b(n) \equiv 0$ and the constant term in the linear transformation always equals zero, we have a concise specific solution as below:
\begin{equation}
\label{eq:b_pos_simple}
g'(pos) =  z_3 z_1^{pos}
\end{equation}

In order to bound Eq.~\ref{eq:final} and Eq.~\ref{eq:b_pos_simple}, the exponential term  $z_1^{pos}$  should have a constrain that $\vert z_1 \vert \leq 1$

% Any complex number with the form  $z_1=\alpha_1 + i \beta_1$ can be transformed into polar plane $z_1=r_1e^{i\theta_1}$. The exponential term can be formulated as
% \begin{equation}
% \label{eq:b_pos_simple}
% \begin{aligned}
% \vert g(pos) \vert &= c_1 \vert z_1^{pos} \vert +c_3 \\
% &= c_1 r^{pos}e^{i\theta_1 pos} + c_3
% \end{aligned}
% \end{equation}


Noting that all the the notations in this appendix including $g,w,z_1,z_2,z_3, \alpha_1,\alpha_2,\alpha_3, \beta_1, \beta_2, \beta_3$ have two implicit superscript $j$ and $d$, corresponding to the word index and the $d$-dimensional for the embedding which are omitted for better reading.





\end{proof}
